# Supplementary material for: Stable Backward Diffusion Models that Minimise Convex Energies
Source: arXiv:1903.03491 ancillary file (2020-06-17)
Supplement: Supplementary file 1 [file supplementary_material.pdf]

# Stable Backward Diffusion Models that Minimise Convex Energies

## – Supplementary Material –

Leif Bergerhoff[1], Marcelo Cárdenas[1], Joachim Weickert[1], and Martin Welk[2]

[1] Mathematical Image Analysis Group,
Faculty of Mathematics and Computer Science,
Saarland University,
Campus E1.7, 66041 Saarbrücken, Germany
{bergerhoff,cardenas,weickert}@mia.uni-saarland.de

[2] Institute of Biomedical Image Analysis,
Private University for Health Sciences, Medical Informatics and Technology,
Eduard-Wallnöfer-Zentrum 1, 6060 Hall/Tyrol, Austria
martin.welk@umit.at

# 1 Derivations

## 1.1 Derivation of Equation (6)

First, Equation (4) can be reformulated as

$$
\begin{aligned}
E(\boldsymbol{v}, \boldsymbol{W}) &= \frac{1}{4} \cdot \sum_{i=1}^{2N} \sum_{j=1}^{2N} w_{i,j} \cdot \Psi((v_j - v_i)^2) \\
&= \frac{1}{4} \cdot \left( \sum_{i=1}^{N} \sum_{j=1}^{2N} w_{i,j} \cdot \Psi((v_j - v_i)^2) + \sum_{i=1}^{N} \sum_{j=1}^{2N} w_{2N+1-i,j} \cdot \Psi((v_j - 2 + v_i)^2) \right) \\
&= \frac{1}{4} \cdot \sum_{i=1}^{N} \sum_{j=1}^{N} \Big( w_{i,j} \cdot \Psi((v_j - v_i)^2) \\
&\qquad + w_{i,2N+1-j} \cdot \Psi((2 - v_j - v_i)^2) \\
&\qquad + w_{2N+1-i,j} \cdot \Psi((v_j - 2 + v_i)^2) \\
&\qquad + w_{2N+1-i,2N+1-j} \cdot \Psi((2 - v_j - 2 + v_i)^2) \Big).
\end{aligned}
$$

Using

$$
\Psi((2+s)^2) = \Psi(s^2) = \Psi((-s)^2),
$$

and

$$
w_{i,\,j} = w_{2N+1-i,\,j} = w_{i,\,2N+1-j} = w_{2N+1-i,\,2N+1-j},
$$

the energy simplifies to

$$
E(\boldsymbol{v}, \boldsymbol{W}) = \frac{1}{2} \cdot \sum_{i=1}^{N} \sum_{j=1}^{N} w_{i,j} \cdot \left( \Psi((v_j - v_i)^2) + \Psi((v_j + v_i)^2) \right).
$$

## 1.2 Positive (Semi-)Definiteness of the Hessian Matrix

Assuming a penaliser function $\Psi(s^2) = \Psi_{a,n}(s^2)$ according to Table 1, the flux function and its derivative read

$$\begin{aligned}\Phi(s) &= a \cdot n \cdot (s-1)^{2n-1},\\ \Phi'(s) &= a \cdot n \cdot (2n-1) \cdot (s-1)^{2n-2}.\end{aligned}$$

Therefore, the entries of the Hessian (9) and (10) adapt to

$$\begin{aligned}\partial_{v_i v_i} E(\boldsymbol{v}, \tilde{\boldsymbol{W}}) &= a \cdot n \cdot (2n-1) \cdot \\ &\quad \Bigg( \sum_{j \in J_2^i} \tilde{w}_{i,j} \cdot \Big( (v_j - v_i - 1)^{2n-2} + (v_j + v_i - 1)^{2n-2} \Big) + \\ &\quad \sum_{j \in J_3^i} \tilde{w}_{i,j} \cdot (v_j + v_i - 1)^{2n-2} \Bigg),\\ \partial_{v_i v_j} E(\boldsymbol{v}, \tilde{\boldsymbol{W}}) &= a \cdot n \cdot (2n-1) \cdot \tilde{w}_{i,j} \cdot \\ &\quad \Big( (v_j + v_i - 1)^{2n-2} - (v_j - v_i - 1)^{2n-2} \Big), \quad \forall j \in J_2^i,\\ \partial_{v_i v_j} E(\boldsymbol{v}, \tilde{\boldsymbol{W}}) &= a \cdot n \cdot (2n-1) \cdot \tilde{w}_{i,j} \cdot (v_j + v_i - 1)^{2n-2}, \quad \forall j \in J_3^i.\end{aligned}$$

Using the Gershgorin circle theorem it is now possible to derive the range of all eigenvalues of the Hessian matrix. The radius of the Gershgorin discs is given by

$$\begin{aligned}r_i &= \sum_{\substack{j=1\\ j \neq i}}^{N} \left| \partial_{v_i v_j} E(\boldsymbol{v}, \tilde{\boldsymbol{W}}) \right| \\ &= a \cdot n \cdot (2n-1) \cdot \\ &\quad \Bigg( \sum_{j \in J_2^i} \tilde{w}_{i,j} \cdot \Big| (v_j + v_i - 1)^{2n-2} - (v_j - v_i - 1)^{2n-2} \Big| + \\ &\quad \sum_{\substack{j \in J_3^i\\ j \neq i}} \tilde{w}_{i,j} \cdot (v_j + v_i - 1)^{2n-2} \Bigg), \qquad \forall i = 1, \ldots, N.\end{aligned}$$

Note that the difference $d_i := \partial_{v_i v_i} E(\boldsymbol{v}, \tilde{\boldsymbol{W}}) - r_i$ fulfils

$$\begin{aligned}d_i &= a \cdot n \cdot (2n-1) \cdot \\ &\quad \Bigg( \sum_{j \in J_2^i} \tilde{w}_{i,j} \cdot \Big( (v_j - v_i - 1)^{2n-2} + (v_j + v_i - 1)^{2n-2} - \\ &\qquad \Big| (v_j + v_i - 1)^{2n-2} - (v_j - v_i - 1)^{2n-2} \Big| \Big) + \\ &\quad \tilde{w}_{i,i} \cdot (2v_i - 1)^{2n-2} \Bigg) \\ &\geq a \cdot n \cdot (2n-1) \cdot \tilde{w}_{i,i} \cdot (2v_i - 1)^{2n-2} \\ &\geq 0, \qquad \forall i = 1, \ldots, N,\end{aligned}$$

where we have used the triangle inequality and the fact that $\tilde{w}_{i,i} > 0$ and $v_i \in (0,1)$. From the theory of Gershgorin it is known that $\lambda_i \geq d_i$ for $1 \leq i \leq N$. Therefore, the eigenvalues of the Hessian are non-negative and the Hessian is positive semi-definite.

*Case* $n = 1$. For $n = 1$ the difference $d_i$ satisfies

$$d_i = a \cdot \left( 2 \cdot \sum_{j \in J_2^i} \tilde{w}_{i,j} + \tilde{w}_{i,i} \right) > 0, \quad \forall i = 1, \ldots, N,$$

since $\tilde{w}_{i,i} > 0$ and as a consequence of $\lambda_i \geq d_i$ for $1 \leq i \leq N$ the Hessian matrix is positive definite.

*Case* $n = 2$. For $n = 2$ the difference $d_i$ reads

$$\begin{aligned} d_i = 6 \cdot n \cdot \Bigg( \sum_{j \in J_2^i} \tilde{w}_{i,j} \cdot \Big( &(v_j - v_i - 1)^2 + (v_j + v_i - 1)^2 \\ &- \left| (v_j + v_i - 1)^2 - (v_j - v_i - 1)^2 \right| \Big) \\ + \tilde{w}_{i,i} \cdot (2v_i - 1)^2 \Bigg)& \\ = 6 \cdot n \cdot \Bigg( \sum_{j \in J_2^i} \tilde{w}_{i,j} \cdot (2v_j^2 + 2v_i^2 - 4v_j + 2 - 4v_i \cdot |v_j - 1|) + \tilde{w}_{i,i} \cdot (2v_i - 1)^2 \Bigg).& \end{aligned}$$

Since $v_j \in (0,1)$ we know that $|v_j - 1| = 1 - v_j$ and we get

$$\begin{aligned} d_i &= 6 \cdot n \cdot \left( 2 \cdot \sum_{j \in J_2^i} \tilde{w}_{i,j} \cdot (v_j^2 + 2v_j v_i + v_i^2 - 2v_j - 2v_i + 1) + \tilde{w}_{i,i} \cdot (2v_i - 1)^2 \right) \\ &= 6 \cdot n \cdot \left( 2 \cdot \sum_{j \in J_2^i} \tilde{w}_{i,j} \cdot \Big( (v_j + v_i)^2 - 2 \cdot (v_j + v_i) + 1 \Big) + \tilde{w}_{i,i} \cdot (2v_i - 1)^2 \right) \\ &= 6 \cdot n \cdot \left( 2 \cdot \sum_{j \in J_2^i} \tilde{w}_{i,j} \cdot (v_j + v_i - 1)^2 + \tilde{w}_{i,i} \cdot (2v_i - 1)^2 \right). \end{aligned}$$

Therefore, if for $1 \leq i \leq N$ at least one of the two conditions

- $v_i \neq \frac{1}{2}$ (since $\tilde{w}_{i,i} > 0$),
- $\exists j \in J_2^i$ with $v_j \neq 1 - v_i$ and $\tilde{w}_{i,j} > 0$,

holds, one can guarantee $\lambda_i \geq d_i > 0$ and thus positive definiteness of the Hessian matrix.

### 1.3 Derivation of Equation (36)

Using $\tilde{\boldsymbol{W}} = \mathbf{1}\mathbf{1}^{\mathrm{T}}$, (4) adapts to

$$\begin{aligned} E(\boldsymbol{v}) &= \frac{1}{4} \cdot \sum_{i=1}^{2N} \sum_{j=1}^{2N} \Psi((v_j - v_i)^2) \\ &= \frac{1}{4} \cdot \left( \sum_{i=1}^{N} \sum_{j=1}^{N} \Psi((v_j - v_i)^2) + \sum_{i=1}^{N} \sum_{j=1}^{N} \Psi((2 - v_j - v_i)^2) \right. \\ &\qquad \left. + \sum_{i=1}^{N} \sum_{j=1}^{N} \Psi((v_j - 2 + v_i)^2) + \sum_{i=1}^{N} \sum_{j=1}^{N} \Psi((2 - v_j - 2 + v_i)^2) \right) \\ &= \frac{1}{2} \cdot \left( \sum_{i=1}^{N} \sum_{j=1}^{N} \Psi((v_j - v_i)^2) + \sum_{i=1}^{N} \sum_{j=1}^{N} \Psi((v_j + v_i)^2) \right). \end{aligned}$$

Splitting the sums into $i < j$, $i = j$, and $i > j$ we get

$$\begin{aligned} E(\boldsymbol{v}) = \frac{1}{2} \cdot \left( \sum_{i=1}^{N-1} \sum_{j=i+1}^{N} \Psi((v_j - v_i)^2) + \sum_{i=1}^{N} \Psi(0) + \sum_{j=1}^{N-1} \sum_{i=j+1}^{N} \Psi((v_j - v_i)^2) \right. \\ \left. + \sum_{i=1}^{N-1} \sum_{j=i+1}^{N} \Psi((v_j + v_i)^2) + \sum_{i=1}^{N} \Psi(4v_i^2) + \sum_{j=1}^{N-1} \sum_{i=j+1}^{N} \Psi((v_j + v_i)^2) \right). \end{aligned}$$

Finally, use $\Phi(0) = 0$, switch $i$ and $j$ in the third term of each row, and use $(v_j - v_i)^2 = (v_i - v_j)^2$ to obtain

$$\begin{aligned} E(\boldsymbol{v}) &= \frac{1}{2} \cdot \left( 2 \cdot \sum_{i=1}^{N-1} \sum_{j=i+1}^{N} \Psi((v_j - v_i)^2) + \sum_{i=1}^{N} \Psi(4v_i^2) \right. \\ &\qquad \left. + 2 \cdot \sum_{i=1}^{N-1} \sum_{j=i+1}^{N} \Psi((v_j + v_i)^2) \right) \\ &= \sum_{i=1}^{N-1} \sum_{j=i+1}^{N} \Psi((v_j - v_i)^2) + \frac{1}{2} \cdot \sum_{i=1}^{N} \Psi(4v_i^2) + \sum_{i=1}^{N-1} \sum_{j=i+1}^{N} \Psi((v_j + v_i)^2). \end{aligned}$$

## 2 Parameters of the Local Model

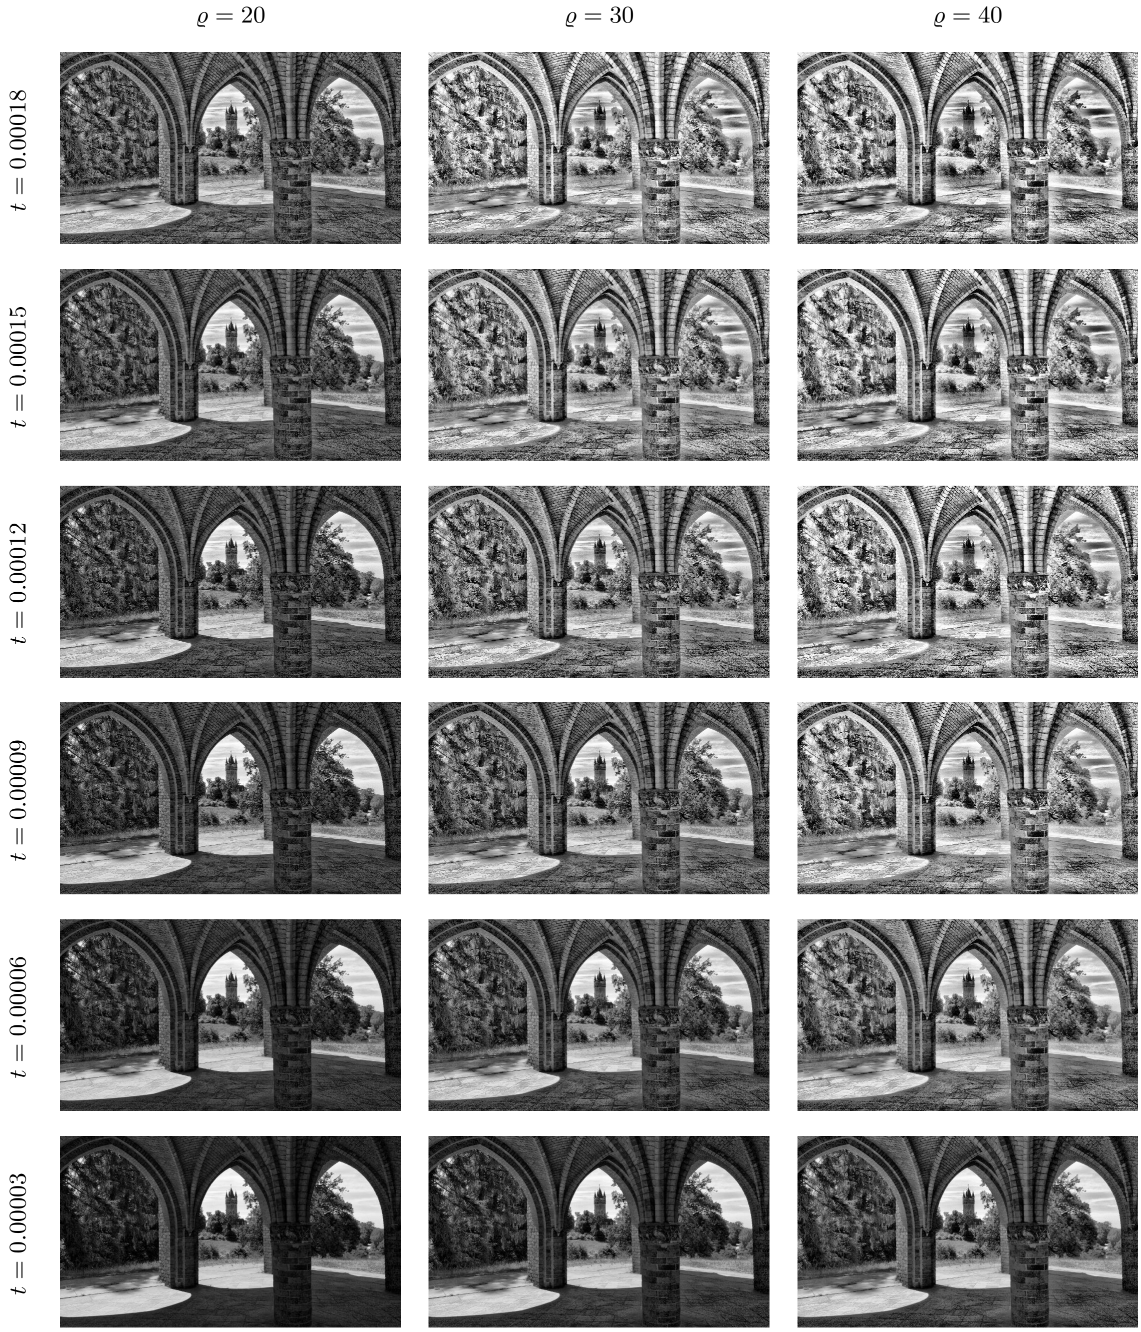


**Fig. 1.** Relation of $t$ and $\varrho$ when applying our model to greyscale images using $\gamma = \gamma_1$. Time increases from bottom to top. Radius increases from left to right.

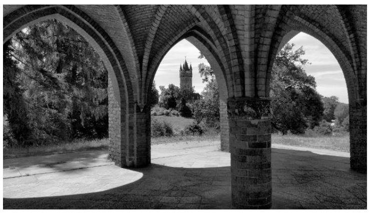

**(a)** $t = 1 \cdot 10^{-5}$.

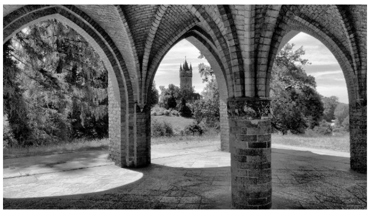

**(b)** $t = 2 \cdot 10^{-5}$.

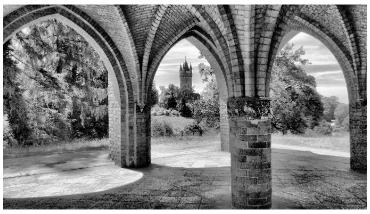

**(c)** $t = 3 \cdot 10^{-5}$.

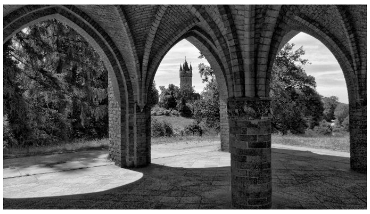

**(d)** $t = 5 \cdot 10^{-5}$.

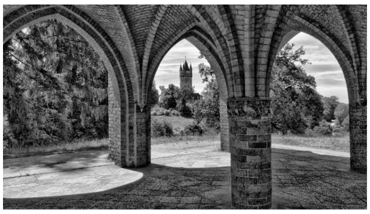

**(e)** $t = 10 \cdot 10^{-5}$.

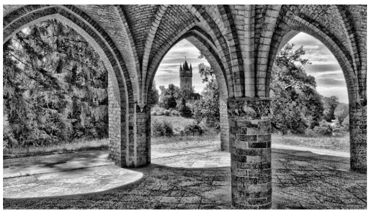

**(f)** $t = 20 \cdot 10^{-5}$.

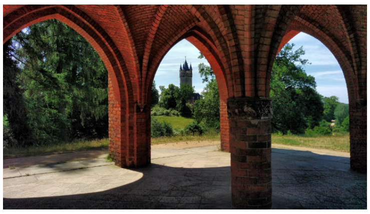

**(g)** $t = 1 \cdot 10^{-5}$.

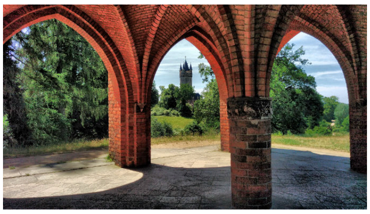

**(h)** $t = 2 \cdot 10^{-5}$.

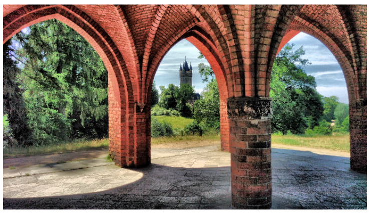

**(i)** $t = 3 \cdot 10^{-5}$.

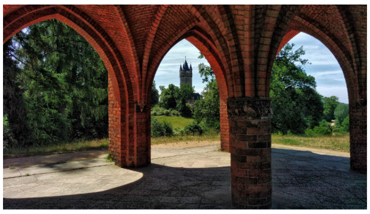

**(j)** $t = 5 \cdot 10^{-5}$.

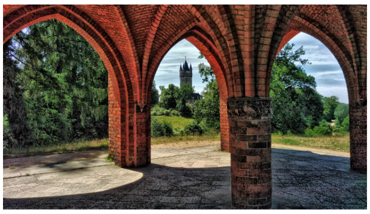

**(k)** $t = 10 \cdot 10^{-5}$.

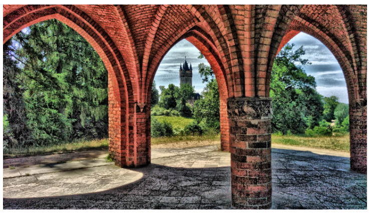

**(l)** $t = 20 \cdot 10^{-5}$.

**Fig. 2.** Influence of the weighting function $\gamma$ when applying our model to greyscale and colour images using $\varrho = 60$ and $\lambda = 0.5$. **(a)-(c):** greyscale input data and $\gamma = \gamma_1$. **(d)-(f):** greyscale input data and $\gamma = \gamma_2$. **(g)-(i):** colour input data and $\gamma = \gamma_1$. **(j)-(l):** colour input data and $\gamma = \gamma_2$.
